# Supplementary material for: Thickness dependence of unidirectional spin-Hall magnetoresistance in metallic bilayers
Source: arXiv:1711.06488 ancillary file (2017-11-17)
Supplement: Supplementary file 1 [file Appendix.pdf]

# Thickness dependence of unidirectional spin-Hall magnetoresistance in metallic bilayers

# Appendix

#### Appendix A: Thermal contributions to the unidirectional spin-Hall magnetoresistance

The USMR is not the only effect that can change the longitudinal resistance of the bilayer structure. If thermal gradients are present in the sample, thermoelectric effects could also contribute to the modulation of the resistance. To measure the thermal contributions separately from the USMR, the second harmonic Hall voltage, $R^{\mathrm{H}}_{2\omega}$ , will be measured instead.

The effects that contribute to the second harmonic Hall resistance are the anomalous Nernst effect (ANE), spin Seebeck effect (SSE), field-like spin-orbit torque (FL-SOT), and anti-damping like spin-orbit torque (AD-SOT).

$$R^{\mathrm{H}}_{2\omega} = R^{\mathrm{H,FL}}_{2\omega}(2\cos\phi^3 - \cos\phi) + (R^{\mathrm{H,ANE+SSE}}_{2\omega} + R^{\mathrm{H,AD}}_{2\omega})\cos\phi, \tag{A.1}$$

where $R^{\mathrm{H,FL}}_{2\omega}$ and $R^{\mathrm{H,AD}}_{2\omega}$ are two coefficients related to the strength of the field-like torque and anti-damping like torque, respectively. $R^{\mathrm{H,ANE+SSE}}_{2\omega}$ is the thermal Hall resistance induced by the ANE and SSE. $\phi$ is the angle between $x$ and $y$ axis.

Since the symmetry of the three terms that make up Equation A.1 are different, the magnitude of $R^{\mathrm{H,FL}}_{2\omega}$ and $R^{\mathrm{H,ANE+SSE}}_{2\omega} + R^{\mathrm{H,AD}}_{2\omega}$ can be determined directly from fitting. The process will be demonstrated in the following part, as exampled by the measurements of a Pt(4)/Co(2)/AlOx(1.15) structure.

The in-plane angular dependence of the second harmonic Hall resistances on the Pt(4)/Co(2)/AlOx(1.15) structures is shown in Figure A.1(a), the resulting signals is a combination of all the effects discussed before. The red line in Figure A.1(a) represent a fit to the data using Equation A.1. For this structure, the fit and data are in excellent agreement.

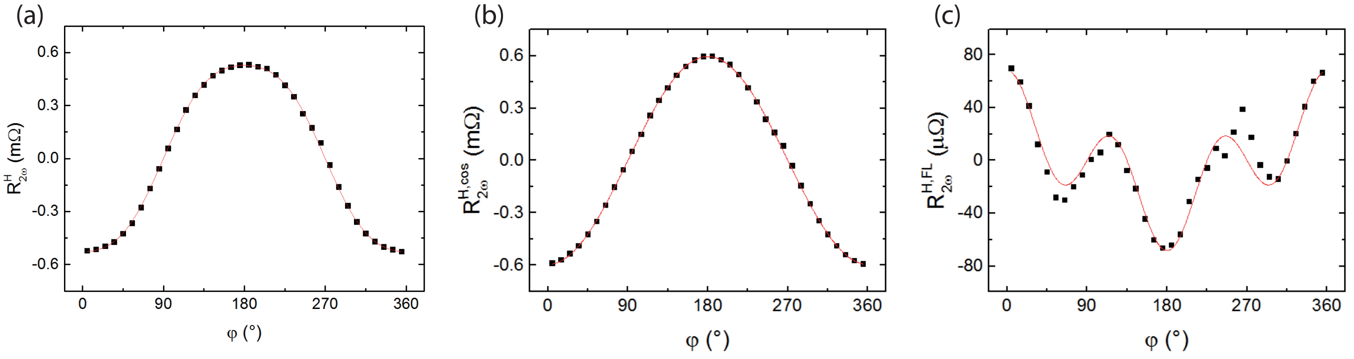


FIG. A.1. (a) Second harmonic Hall resistance for a Pt/Co(20 nm) structure, measured at $B_{\mathrm{ext}} = 547.5$ mT. The red line is a fit using Equation A.1. (b) $\cos\varphi$ contribution to the second harmonic Hall resistance of the 2 nm sample. (c) FL-SOT contribution to the second harmonic Hall resistance. In all three figures, the error bars for each data point are too small to be seen.

Using the magnitudes gathered from the fit, the second harmonic Hall resistance can be separated into the individual components. In Figure A.1(b) the FL-SOT contribution has been removed from $R^{H}_{2\omega}$, resulting in the $\cos\varphi$ contribution. The red line is a fit with a pure cosine function, that shows excellent agreement with the data. In Figure A.1(c), the $\cos\varphi$ contribution has been removed from $R^{H}_{2\omega}$. The red line represent a $2\cos\phi^3 - \cos\phi$ fit to the data; the data fits the theoretically predicted signal well.

The magnitude of the FL-SOT contribution is now known, although the ANE and SSE effects are still mixed together with the AD-SOT signal. To further separate the ANE, SSE and AD-SOT the second harmonic Hall resistance is measured as a function of the external field. The thermoelectric effects are expected to be constant with respect to

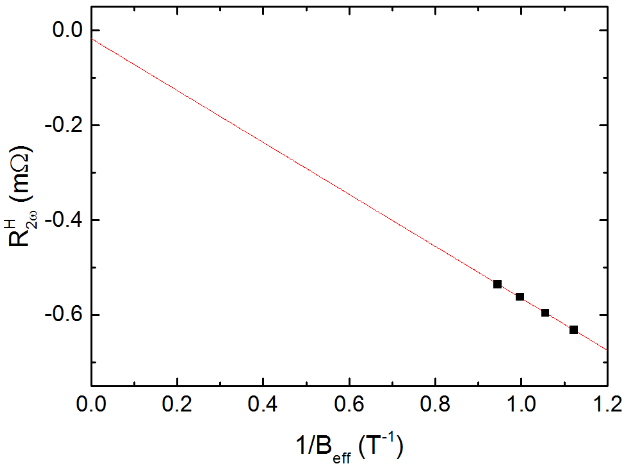


FIG. A.2. Field dependence of the $\cos\varphi$ contribution to the second harmonic Hall resistance of a Pt/Co(2 nm) bilayer structure.

changes in the external field magnitude, whereas the AD-SOT contribution should decrease for increasing field[4]. To this end, the measurement discussed above is repeated for different field magnitudes between 490 and 660 mT. These fields are chosen to ensure that the magnetization is saturated along the external field. The resulting measurement points can be plotted versus the inverse external field $\frac{1}{B_{\text{eff}}}$ and linearly fitted in Figure A.2.. The slope of the resulting linear function scales with $R_{2\omega}^{\text{H,AD}}$ and the intercept with the y-axis is equal to $R_{2\omega}^{\text{H,ANE+SSE}}$. The ANE and SSE cannot be separated further, since the symmetries of their signal are the same, but the magnitude of the thermal contributions to the second harmonic Hall resistance can be determined using this method.

Using the fit, the magnitude of the ANE and SSE contributions can be calculated. The combined contribution from the ANE and SSE is found to be, $R_{2\omega}^{\text{H,ANE+SSE}} = 17 \pm 2\ \mu\Omega$. Avci et al.[4] found a ANE and SSE contribution of 20 $\mu\Omega$, which is very close to the one found here.

As the objective is to determine the contributions of the thermoelectric effects to the USMR signal, the thermal contributions to the longitudinal second harmonic resistance have to be calculated. Since the origin of the ANE and SSE is microscopic, the signals are proportional to the distance over which they are measured. Therefore the ratio between the longitudinal and Hall contributions is equal to the length ratio of the Hall bar ($l = 20\ \mu$m, $w = 5\ \mu$m):

$$R_{2\omega}^{\text{ANE+SSE}} = \frac{l}{w} R_{2\omega}^{\text{H,ANE+SSE}} = 68 \pm 8 \quad \mu\Omega. \tag{A.2}$$

The measured USMR signal for the Pt(4 nm)/Co(2 nm) structure to be around 2.19 mΩ. Thus, the thermal contribution to the USMR is approximately 3%, which is negligibly small. To determine if the thickness dependence of the thermal contributions, the measurements described above have been repeated for more cobalt layer thicknesses. The final result is shown in Fig. 2(a) in the main text.
